# Supplementary material for: Hot carrier dynamics in plasmonic transition metal nitrides
Source: arXiv:1802.00727 source file (2018-05-02)
Supplement: Supplementary file 1 [file SI.pdf]

# Supplemental Information for:
# "Hot carrier dynamics in plasmonic transition metal nitrides"

Adela Habib,[1] Fred Florio,[1] and Ravishankar Sundararaman[1, 2]

[1]*Department of Physics, Applied Physics and Astronomy, Rensselaer Polytechnic Institute, Troy, NY 12180, USA*
[2]*Department of Materials Science and Engineering, Rensselaer Polytechnic Institute, Troy, NY 12180, USA*

(Dated: February 1, 2018)

The figures in this supplementary information show calculated band structures and density of states of both electrons and phonons for all group IV, V and VI nitride structures discussed in the main text.

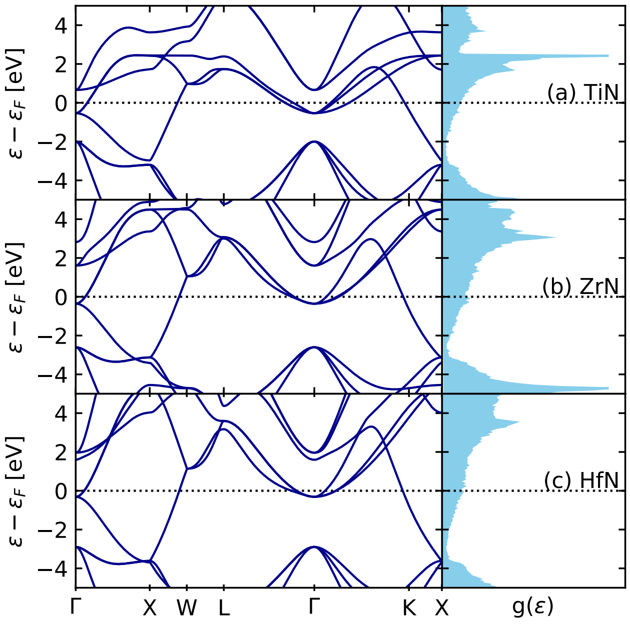


FIG. 1. Electronic band structure and density of states for rock-salt group IV nitrides.

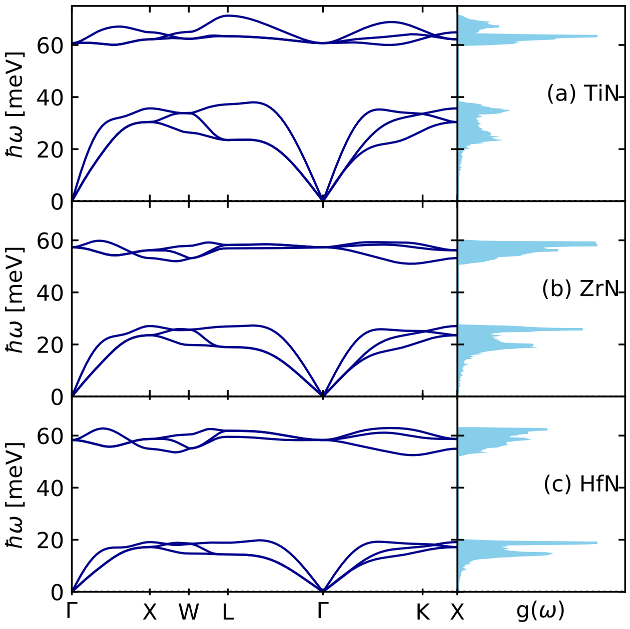


FIG. 2. Phonon band structure and density of states for rock-salt group IV nitrides.

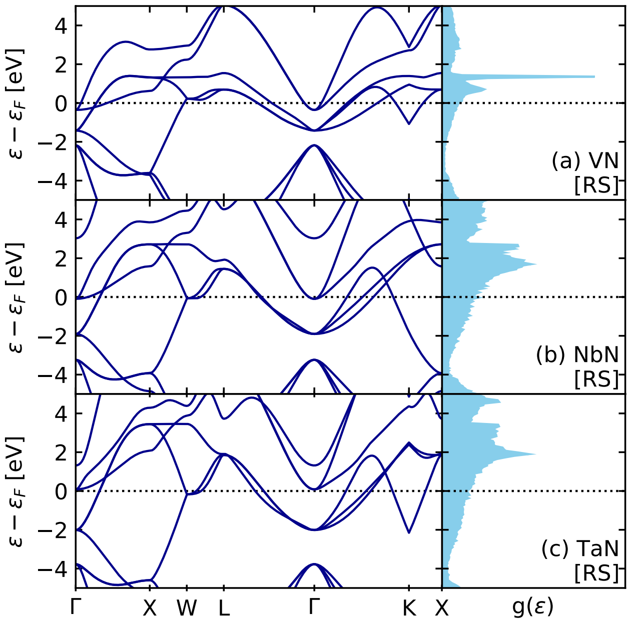


FIG. 3. Electronic band structure and density of states for rock-salt group V nitrides.

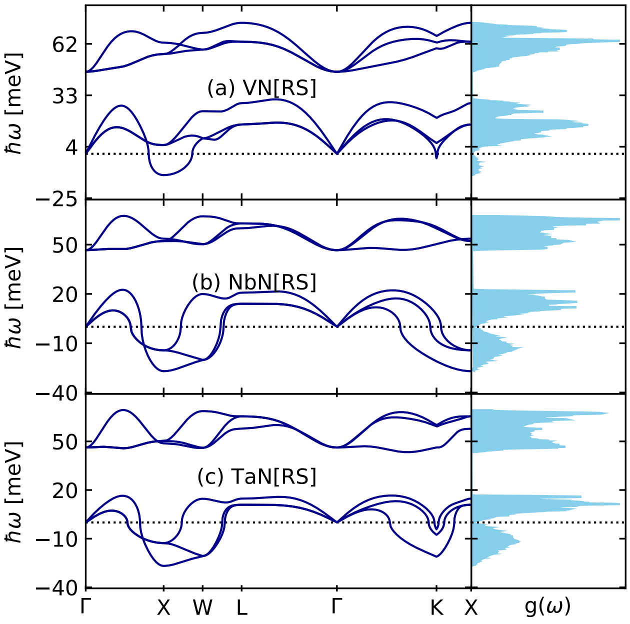


FIG. 4. Phonon band structure and density of states for rock-salt group V nitrides. Imaginary phonon frequencies indicate that this structure is not mechanically stable at zero temperature for this group.

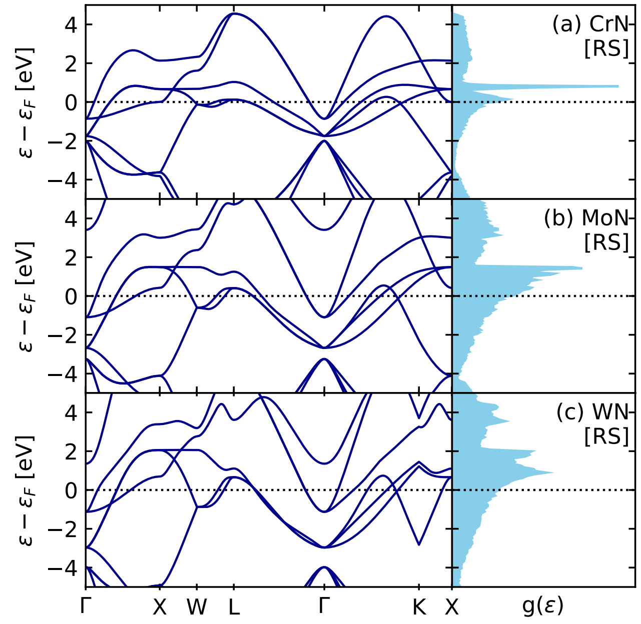


FIG. 5. Electronic band structure and density of states for rock-salt group VI nitrides.

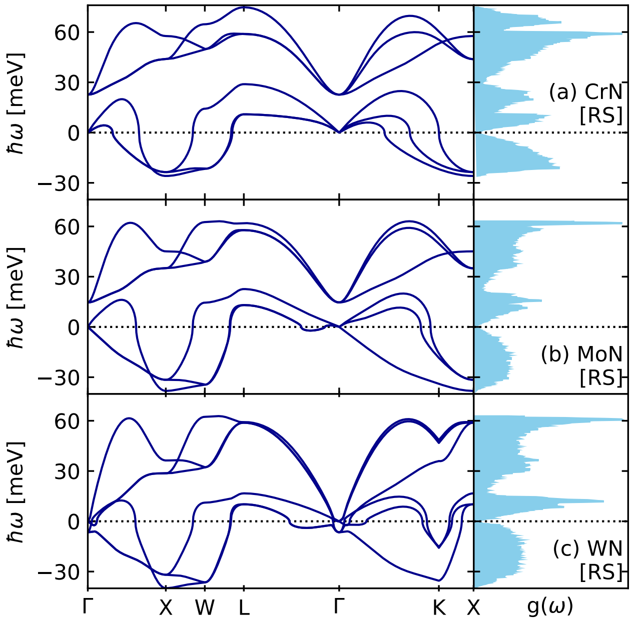


FIG. 6. Phonon band structure and density of states for rock-salt group VI nitrides. Imaginary phonon frequencies indicate that this structure is not mechanically stable at zero temperature for this group.

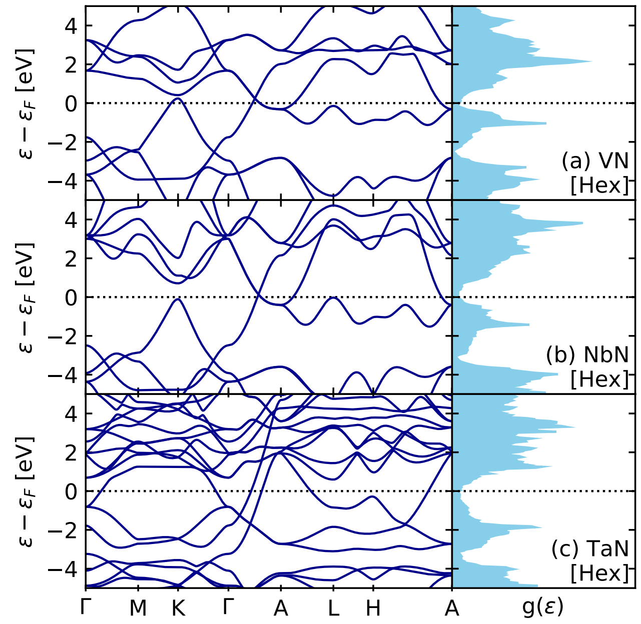


FIG. 7. Electronic band structure and density of states for hexagonal group V nitrides. The Fermi energy is in a minimum of density of states, resulting in the uniquely high electron-phonon relaxation times of these materials.

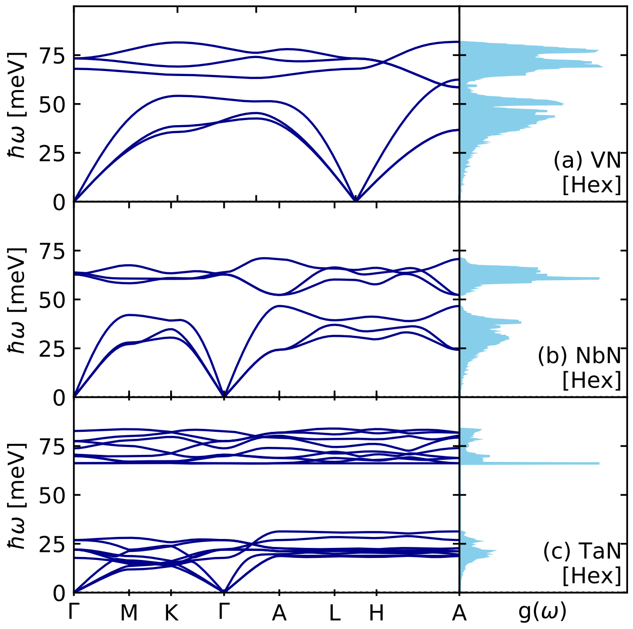


FIG. 8. Phonon band structure and density of states for hexagonal group V nitrides.

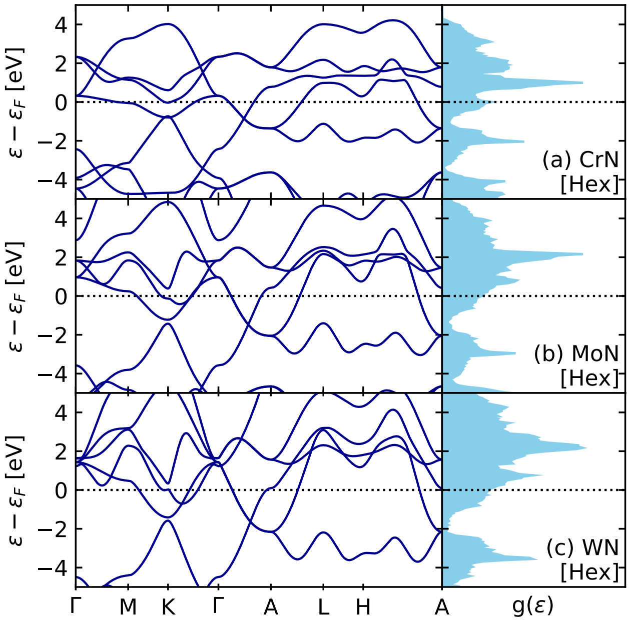


FIG. 9. Electronic band structure and density of states for hexagonal group VI nitrides.

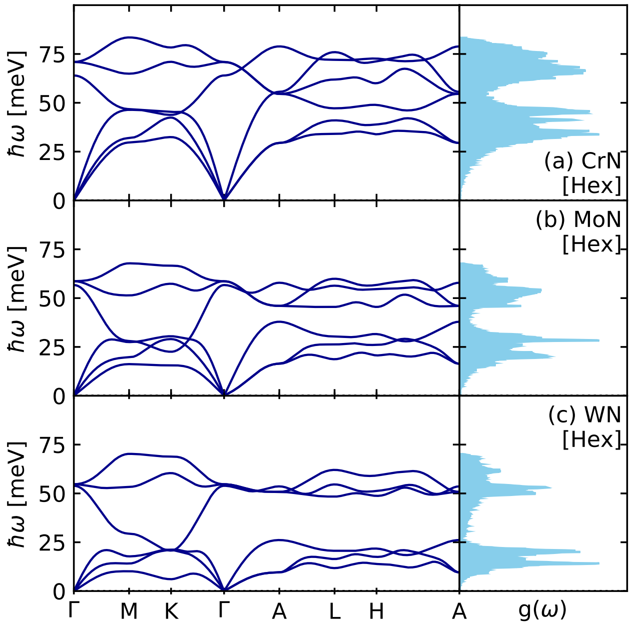


FIG. 10. Phonon band structure and density of states for hexagonal group VI nitrides.

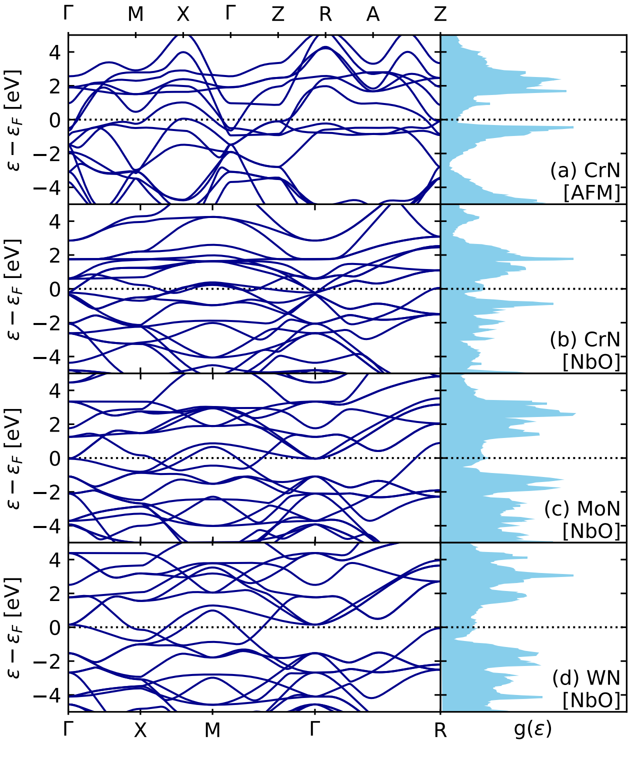


FIG. 11. Electronic band structure and density of states for AFM / NbO-structure group VI nitrides.

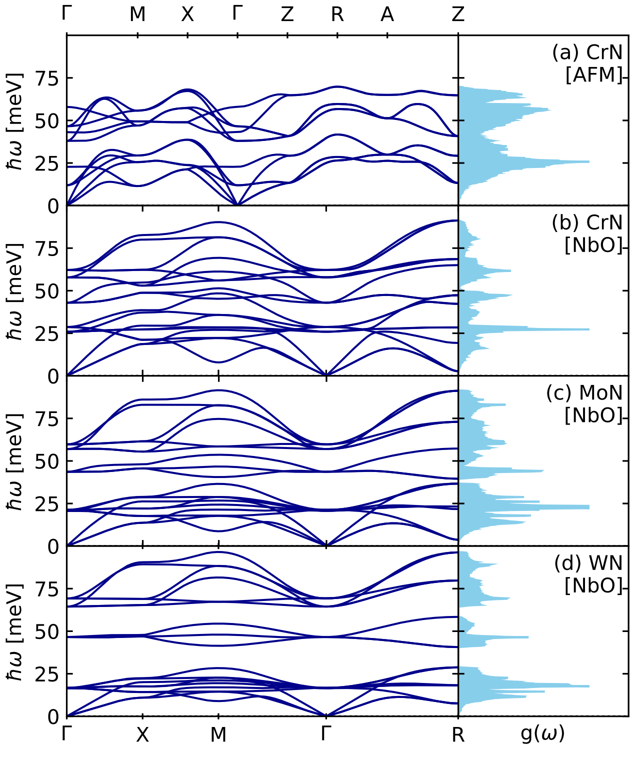


FIG. 12. Phonon band structure and density of states for AFM / NbO-structure group VI nitrides.

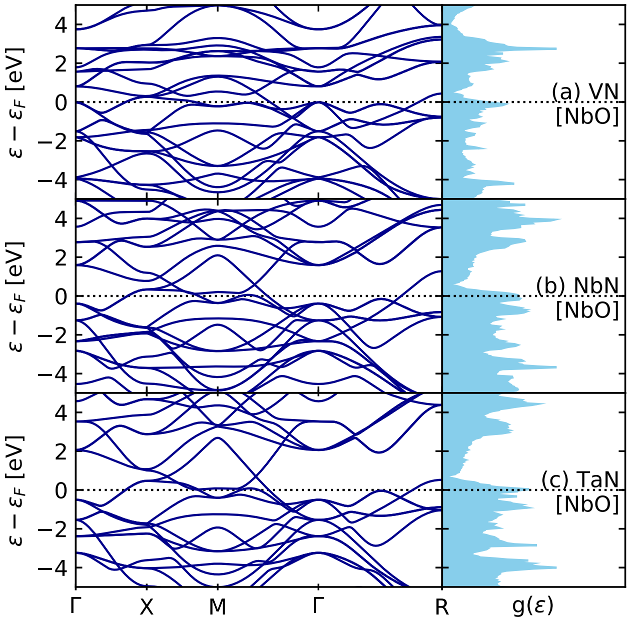


FIG. 13. Electronic band structure and density of states for NbO-structure group V nitrides.

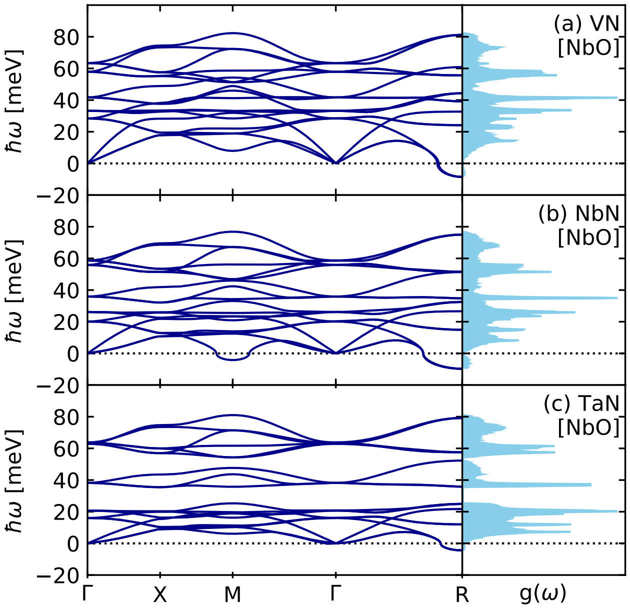


FIG. 14. Phonon band structure and density of states for NbO-structure group V nitrides. Imaginary phonon frequencies indicate that this structure is not mechanically stable at zero temperature for this group.
